# Supplementary material for: Selecting Walk Schemes for Database Embedding
Source: arXiv:2401.11215 source file (2024-01-20)
Supplement: Supplementary file 1 [file section_appendix.tex]

%\newpage
\appendix

\begin{figure*}
\ifx\QUICK\undefined
%begin 1 world
\centering
\rotatebox[origin=t]{90}{\small~\textbf{World}}
\begin{subfigure}{0.155\textwidth}
    \caption*{\textbf{\kvar}}
    \resizebox{\linewidth}{!}{\input{plots/pgf_plots/world_k_var.tex}}
    %\caption{Time}
    \label{fig:first}
\end{subfigure}
\hfill
\begin{subfigure}{0.155\textwidth}
    \caption*{\textbf{\mi}}
    \resizebox{\linewidth}{!}{\input{plots/pgf_plots/world_MI.tex}}
    %\caption{Time}
    \label{fig:second}
\end{subfigure}
\hfill
\begin{subfigure}{0.155\textwidth}
    \caption*{\textbf{\oneepoch}}
    \resizebox{\linewidth}{!}{\input{plots/pgf_plots/world_1ep.tex}}
    %\caption{Time}
    \label{fig:third}
\end{subfigure}
\hfill
\begin{subfigure}{0.155\textwidth}
    \caption*{\textbf{\length}}
    \resizebox{\linewidth}{!}{\input{plots/pgf_plots/world_len.tex}}
    %\caption{Time}
    \label{fig:third4}
\end{subfigure}
\hfill
\begin{subfigure}{0.155\textwidth}
    \caption*{\textbf{\random}}
    \resizebox{\linewidth}{!}{\input{plots/pgf_plots/world_random.tex}}
    %\caption{Time}
    \label{fig:third5}
\end{subfigure}
\hfill
\begin{subfigure}{0.155\textwidth}
    \caption*{\textbf{\sampling}}
    \resizebox{\linewidth}{!}{\input{plots/pgf_plots/world_sampling.tex}}
    %\caption{Time}
    \label{fig:third6}
\end{subfigure}
%end 1 world

%begin 2 genes
\centering
\rotatebox[origin=t]{90}{\small~\textbf{Genes}}
\begin{subfigure}{0.155\textwidth}
    \resizebox{\linewidth}{!}{\input{plots/pgf_plots/genes_k_var.tex}}
    %\label{fig:first}
\end{subfigure}
\hfill
\begin{subfigure}{0.155\textwidth}
    \resizebox{\linewidth}{!}{\input{plots/pgf_plots/genes_MI.tex}}
    %\label{fig:second}
\end{subfigure}
\hfill
\begin{subfigure}{0.155\textwidth}
    \resizebox{\linewidth}{!}{\input{plots/pgf_plots/genes_1ep.tex}}
    %\label{fig:third}
\end{subfigure}
\hfill
\begin{subfigure}{0.155\textwidth}
    \resizebox{\linewidth}{!}{\input{plots/pgf_plots/genes_len.tex}}
    %\label{fig:third4}
\end{subfigure}
\hfill
\begin{subfigure}{0.155\textwidth}
    \resizebox{\linewidth}{!}{\input{plots/pgf_plots/genes_random.tex}}
    %\label{fig:third5}
\end{subfigure}
\hfill
\begin{subfigure}{0.155\textwidth}
    \resizebox{\linewidth}{!}{\input{plots/pgf_plots/genes_sampling.tex}}
    %\label{fig:third6}
\end{subfigure}
%end 2 genes

%begin 3 mondial_religion
\centering
\rotatebox[origin=t]{90}{\small~\textbf{M-Religion}} %Acc-mondial_religion
\begin{subfigure}{0.155\textwidth}
    \resizebox{\linewidth}{!}{\input{plots/pgf_plots/mondial_religion_k_var.tex}}
    %\label{fig:first}
\end{subfigure}
\hfill
\begin{subfigure}{0.155\textwidth}
    \resizebox{\linewidth}{!}{\input{plots/pgf_plots/mondial_religion_MI}}
    %\label{fig:second}
\end{subfigure}
\hfill
\begin{subfigure}{0.155\textwidth}
    \resizebox{\linewidth}{!}{\input{plots/pgf_plots/mondial_religion_1ep.tex}}
    %\label{fig:third}
\end{subfigure}
\hfill
\begin{subfigure}{0.155\textwidth}
    \resizebox{\linewidth}{!}{\input{plots/pgf_plots/mondial_religion_len.tex}}
    %\label{fig:third4}
\end{subfigure}
\hfill
\begin{subfigure}{0.155\textwidth}
    \resizebox{\linewidth}{!}{\input{plots/pgf_plots/mondial_religion_random.tex}}
    %\label{fig:third5}
\end{subfigure}
\hfill
\begin{subfigure}{0.155\textwidth}
    \resizebox{\linewidth}{!}{\input{plots/pgf_plots/mondial_religion_sampling.tex}}
    %\label{fig:third6}
\end{subfigure}
%end 3 mondial_religion

%begin 4 mondial_continent
\centering
\rotatebox[origin=t]{90}{\small~\textbf{M-Continent}} %
\begin{subfigure}{0.155\textwidth}
    \resizebox{\linewidth}{!}{\input{plots/pgf_plots/mondial_continent_k_var.tex}}
    \caption*{\textbf{Time} (sec)}
    %\label{fig:first}
\end{subfigure}
\hfill
\begin{subfigure}{0.155\textwidth}
    \resizebox{\linewidth}{!}{\input{plots/pgf_plots/mondial_continent_MI}}
    \caption*{\textbf{Time} (sec)}
    %\label{fig:second}
\end{subfigure}
\hfill
\begin{subfigure}{0.155\textwidth}
    \resizebox{\linewidth}{!}{\input{plots/pgf_plots/mondial_continent_1ep.tex}}
    \caption*{\textbf{Time} (sec)}
    %\label{fig:third}
\end{subfigure}
\hfill
\begin{subfigure}{0.155\textwidth}
    \resizebox{\linewidth}{!}{\input{plots/pgf_plots/mondial_continent_len.tex}}
    \caption*{\textbf{Time} (sec)}
    %\label{fig:third4}
\end{subfigure}
\hfill
\begin{subfigure}{0.155\textwidth}
    \resizebox{\linewidth}{!}{\input{plots/pgf_plots/mondial_continent_random.tex}}
    \caption*{\textbf{Time} (sec)}
    %\label{fig:third5}
\end{subfigure}
\hfill
\begin{subfigure}{0.155\textwidth}
    \resizebox{\linewidth}{!}{\input{plots/pgf_plots/mondial_continent_sampling.tex}}
    \caption*{\textbf{Time} (sec)}
    %\label{fig:third6}
\end{subfigure}
%end 4 mondial_continent

\caption{The performance on the downstream task as a function of time for different ratios of targeted walk schemes used for training. More precisely, in the end of each training epoch of \forward we record the time (x-axis) and the accuracy of the downstream task (y-axis).
\label{fig:selected_graphs_time_acc_vis1}}

\end{figure*}

%%%%%%%%%%%%%%%%%%%%%%%%%%%%%%%%%%%%%%%%%%%%%%%%%%%%%%%%%%%%%%%%%%%%%%%%%%%%%%%%%%%%%%%%%%%%%%%%%%%%%%%%%%%%%%%%%%%%%%%%%%%%%%%%%%%%%%%%%%%%%%%%%%%%%%%%%%%%%%%%%%%%%%%%%%%%%%%%%%%%%%%%%%%%%%%%%%%%%%%%%%%%%%%%%%%%%%

\begin{figure*}
%begin 5 mondial_inflation
\centering
\rotatebox[origin=t]{90}{\small~\textbf{M-Inflation}} %Acc-mondial_inflation
\begin{subfigure}{0.155\textwidth}
    \caption*{\textbf{\kvar}}
    \resizebox{\linewidth}{!}{\input{plots/pgf_plots/mondial_inflation_k_var.tex}}
    %\label{fig:first}
\end{subfigure}
\hfill
\begin{subfigure}{0.155\textwidth}
    \caption*{\textbf{\mi}}
    \resizebox{\linewidth}{!}{\input{plots/pgf_plots/mondial_inflation_MI}}
    %\label{fig:second}
\end{subfigure}
\hfill
\begin{subfigure}{0.155\textwidth}
    \caption*{\textbf{\oneepoch}}
    \resizebox{\linewidth}{!}{\input{plots/pgf_plots/mondial_inflation_1ep.tex}}
    %\label{fig:third}
\end{subfigure}
\hfill
\begin{subfigure}{0.155\textwidth}
    \caption*{\textbf{\length}}
    \resizebox{\linewidth}{!}{\input{plots/pgf_plots/mondial_inflation_len.tex}}
    %\label{fig:third4}
\end{subfigure}
\hfill
\begin{subfigure}{0.155\textwidth}
    \caption*{\textbf{\random}}
    \resizebox{\linewidth}{!}{\input{plots/pgf_plots/mondial_inflation_random.tex}}
    %\label{fig:third5}
\end{subfigure}
\hfill
\begin{subfigure}{0.155\textwidth}
    \caption*{\textbf{\sampling}}
    \resizebox{\linewidth}{!}{\input{plots/pgf_plots/mondial_inflation_sampling.tex}}
    %\label{fig:third6}
\end{subfigure}
%end 5 mondial_inflation

%begin 6 hepatitis
\centering
\rotatebox[origin=t]{90}{\small~\textbf{Hepatitis}}
\begin{subfigure}{0.155\textwidth}
    \resizebox{\linewidth}{!}{\input{plots/pgf_plots/hepatitis_k_var.tex}}
    %\label{fig:first}
\end{subfigure}
\hfill
\begin{subfigure}{0.155\textwidth}
    \resizebox{\linewidth}{!}{\input{plots/pgf_plots/hepatitis_MI}}
    %\label{fig:second}
\end{subfigure}
\hfill
\begin{subfigure}{0.155\textwidth}
    \resizebox{\linewidth}{!}{\input{plots/pgf_plots/hepatitis_1ep.tex}}
    %\label{fig:third}
\end{subfigure}
\hfill
\begin{subfigure}{0.155\textwidth}
    \resizebox{\linewidth}{!}{\input{plots/pgf_plots/hepatitis_len.tex}}
    %\label{fig:third4}
\end{subfigure}
\hfill
\begin{subfigure}{0.155\textwidth}
    \resizebox{\linewidth}{!}{\input{plots/pgf_plots/hepatitis_random.tex}}
    %\label{fig:third5}
\end{subfigure}
\hfill
\begin{subfigure}{0.155\textwidth}
    \resizebox{\linewidth}{!}{\input{plots/pgf_plots/hepatitis_sampling.tex}}
    %\label{fig:third6}
\end{subfigure}
%end 6 hepatitis

%begin 7 mondial_infant-mortality
\centering
\rotatebox[origin=t]{90}{\small~\textbf{M-Infant Mort.}} %Acc-mondial_infant-mortality
\begin{subfigure}{0.155\textwidth}
    \resizebox{\linewidth}{!}{\input{plots/pgf_plots/mondial_infant-mortality_k_var.tex}}
    %\label{fig:first}
\end{subfigure}
\hfill
\begin{subfigure}{0.155\textwidth}
    \resizebox{\linewidth}{!}{\input{plots/pgf_plots/mondial_infant-mortality_MI}}
    %\label{fig:second}
\end{subfigure}
\hfill
\begin{subfigure}{0.155\textwidth}
    \resizebox{\linewidth}{!}{\input{plots/pgf_plots/mondial_infant-mortality_1ep.tex}}
    %\label{fig:third}
\end{subfigure}
\hfill
\begin{subfigure}{0.155\textwidth}
    \resizebox{\linewidth}{!}{\input{plots/pgf_plots/mondial_infant-mortality_len.tex}}
    %\label{fig:third4}
\end{subfigure}
\hfill
\begin{subfigure}{0.155\textwidth}
    \resizebox{\linewidth}{!}{\input{plots/pgf_plots/mondial_infant-mortality_random.tex}}
    %\label{fig:third5}
\end{subfigure}
\hfill
\begin{subfigure}{0.155\textwidth}
    \resizebox{\linewidth}{!}{\input{plots/pgf_plots/mondial_infant-mortality_sampling.tex}}
    %\label{fig:third6}
\end{subfigure}
%end 7 mondial_infant-mortality

%begin 8 mondial_GDP
\centering
\rotatebox[origin=t]{90}{\small~\textbf{M-GDP}} %Acc-mondial_GDP
\begin{subfigure}{0.155\textwidth}
    \resizebox{\linewidth}{!}{\input{plots/pgf_plots/mondial_GDP_k_var.tex}}
    %\label{fig:first}
\end{subfigure}
\hfill
\begin{subfigure}{0.155\textwidth}
    \resizebox{\linewidth}{!}{\input{plots/pgf_plots/mondial_GDP_MI}}
    %\label{fig:second}
\end{subfigure}
\hfill
\begin{subfigure}{0.155\textwidth}
    \resizebox{\linewidth}{!}{\input{plots/pgf_plots/mondial_GDP_1ep.tex}}
    %\label{fig:third}
\end{subfigure}
\hfill
\begin{subfigure}{0.155\textwidth}
    \resizebox{\linewidth}{!}{\input{plots/pgf_plots/mondial_GDP_len.tex}}
    %\label{fig:third4}
\end{subfigure}
\hfill
\begin{subfigure}{0.155\textwidth}
    \resizebox{\linewidth}{!}{\input{plots/pgf_plots/mondial_GDP_random.tex}}
    %\label{fig:third5}
\end{subfigure}
\hfill
\begin{subfigure}{0.155\textwidth}
    \resizebox{\linewidth}{!}{\input{plots/pgf_plots/mondial_GDP_sampling.tex}}
    %\label{fig:third6}
\end{subfigure}
%end 8 mondial_GDP

%begin 9 last mutagenesis
\rotatebox[origin=t]{90}{\small~\textbf{Mutagenesis}} 
\begin{subfigure}{0.155\textwidth}
    \resizebox{\linewidth}{!}{\input{plots/pgf_plots/mutagenesis_k_var.tex}}
    \caption*{\textbf{Time} (sec)}
    \label{fig:2first}
\end{subfigure}
\hfill
\begin{subfigure}{0.155\textwidth}
    \resizebox{\linewidth}{!}{\input{plots/pgf_plots/mutagenesis_MI.tex}}
    \caption*{\textbf{Time} (sec)}
    \label{fig:2second}
\end{subfigure}
\hfill
\begin{subfigure}{0.155\textwidth}
    \resizebox{\linewidth}{!}{\input{plots/pgf_plots/mutagenesis_1ep}}
    \caption*{\textbf{Time} (sec)}
    \label{fig:2third}
\end{subfigure}
\hfill
\begin{subfigure}{0.155\textwidth}
    \resizebox{\linewidth}{!}{\input{plots/pgf_plots/mutagenesis_len.tex}}
    \caption*{\textbf{Time} (sec)}
    \label{fig:2third4}
\end{subfigure}
\hfill
\begin{subfigure}{0.155\textwidth}
    \resizebox{\linewidth}{!}{\input{plots/pgf_plots/mutagenesis_random.tex}}
    \caption*{\textbf{Time} (sec)}
    \label{fig:2third5}
\end{subfigure}
\hfill
\begin{subfigure}{0.155\textwidth}
    \resizebox{\linewidth}{!}{\input{plots/pgf_plots/mutagenesis_sampling.tex}}
    \caption*{\textbf{Time} (sec)}
    \label{fig:2third6}
\end{subfigure}
\else\QUICK
\fi
\caption{The performance on the downstream task as a function of time for different ratios of targeted walk schemes used for training. More precisely, in the end of each training epoch of \forward we record the time (x-axis) and the accuracy of the downstream task (y-axis).
\label{fig:selected_graphs_time_acc_vis2}}
\end{figure*}

\section{Additional Experiments} \label{appendix:Additional Experiments}

%\ylinline{Here the mega figure is referenced}
%\ylinline{Talk about what we can see in the figure}
%\ylinline{talk about mutagenesis MI that is shifted}

Figure~\ref{fig:selected_graphs_time_acc_vis1} and~\ref{fig:selected_graphs_time_acc_vis2} provide the full results of the experiment in Section~\ref{sec:exp:results-individual} for all strategies and downstream tasks.
The plot the learning curves for different ratios of targeted walk schemes that are retained for training.
These full results were omitted in the main part to save space.
%In this section, we give experimental results for all datasets, tasks, and strategy considered in the paper. The experiments are similar to those of , and are shown in.

Note that when using \mi on the mutagenesis dataset, preprocessing (i.e. the mutual information calculation) takes a significant amount of time. 
For that reason, in this specific plot we ran the embedding for more time and didn't plot the original \forward run, which takes less time to train then the entire preprocessing of this experiments.
